# Supplementary material for: Variationally Optimized Free Energy Flooding for Rate Calculation
Source: arXiv:1506.02545 ancillary file (2015-06-18)
Supplement: Supplementary file 1 [file SupplementalMaterial_Archive_6-8-2015.pdf]

# Supplemental Material for arXiv “Variationally Optimized Free Energy Flooding for Rate Calculation”

James McCarty,<sup>1</sup> Omar Valsson,<sup>1,2</sup> Pratyush Tiwary,<sup>3</sup> and Michele Parrinello<sup>1,2,\*</sup>

<sup>1</sup>*Department of Chemistry and Applied Biosciences, ETH Zurich and Facoltà di Informatica,  
Istituto di Scienze Computationali, Università della Svizzera italiana,  
Via Giuseppe Buffi 13, CH-6900, Lugano, Switzerland.*

<sup>2</sup>*National Center for Computational Design and Discovery of Novel Materials MARVEL.*

<sup>3</sup>*Department of Chemistry, Columbia University, New York, NY 10027.*

(Dated: June 9, 2015)

---

\*Electronic address: [parrinello@phys.chem.ethz.ch](mailto:parrinello@phys.chem.ethz.ch)

This Supplemental Material contains details of the optimization procedure for the bias, computational protocols employed in the main text, and supporting information regarding the methods used.

### S1. STOCHASTIC OPTIMIZATION OF THE BIAS POTENTIAL

In this section we discuss the details of the optimization of the bias potential, defined in the main text as,

$$V(\mathbf{s}) = v(\mathbf{s})\mathcal{S}(-v(\mathbf{s}) - F_c) \quad (\text{S1})$$

We begin by writing the function,  $v(\mathbf{s})$  as a linear expansion in terms of a set of basis functions,  $f_k(\mathbf{s})$ ,

$$v(\mathbf{s}) = v(\mathbf{s}; \alpha) = \sum_k \alpha_k \cdot f_k(\mathbf{s}), \quad (\text{S2})$$

so that the bias,  $V(\mathbf{s})$  depends on  $\{\alpha_k\}$  from Eq. S1,

$$V(\mathbf{s}; \alpha) = v(\mathbf{s}; \alpha)\mathcal{S}(-v(\mathbf{s}; \alpha) - F_c) \quad (\text{S3})$$

We minimize the functional,

$$\Omega[V] = \frac{1}{\beta} \log \frac{\int d\mathbf{s} e^{-\beta[F(\mathbf{s})+V(\mathbf{s})]}}{\int d\mathbf{s} e^{-\beta F(\mathbf{s})}} + \int d\mathbf{s} p(\mathbf{s})V(\mathbf{s}), \quad (\text{S4})$$

with respect to the  $\{\alpha_k\}$  variational parameters by employing the gradient,

$$\frac{\partial \Omega(\alpha)}{\partial \alpha_k} = - \left\langle \frac{\partial V(\mathbf{s}; \alpha)}{\partial \alpha_k} \right\rangle_V + \left\langle \frac{\partial V(\mathbf{s}; \alpha)}{\partial \alpha_k} \right\rangle_p \quad (\text{S5})$$

and Hessian matrix,  $H_{kk'}$ ,

$$H_{k,k'} = \beta \cdot \text{Cov} \left[ \frac{\partial V(\mathbf{s}; \alpha)}{\partial \alpha_k}, \frac{\partial V(\mathbf{s}; \alpha)}{\partial \alpha_{k'}} \right]_V - \left\langle \frac{\partial^2 V(\mathbf{s}; \alpha)}{\partial \alpha_k \partial \alpha_{k'}} \right\rangle_V + \left\langle \frac{\partial^2 V(\mathbf{s}; \alpha)}{\partial \alpha_k \partial \alpha_{k'}} \right\rangle_p, \quad (\text{S6})$$

where the expectation values indicate ensemble averages in either a biased ensemble with bias,  $V(\mathbf{s})$ , or over the target distribution ensemble with normalized probability distribution,  $p(\mathbf{s})$ , and  $\text{Cov}[\dots]_V$  is the covariance obtained in a biased simulation. In general the switching function comes into the derivatives in Eq. S5 as

$$\frac{\partial V(\mathbf{s}; \alpha)}{\partial \alpha_k} = \mathcal{S}(-v(\mathbf{s}; \alpha) - F_c) \frac{\partial v(\mathbf{s}; \alpha)}{\partial \alpha_k} + v(\mathbf{s}; \alpha) \frac{\partial \mathcal{S}(-v(\mathbf{s}; \alpha) - F_c)}{\partial \alpha_k}, \quad (\text{S7})$$

which after the chain rule, becomes,

$$\frac{\partial V(\mathbf{s}; \alpha)}{\partial \alpha_k} = \frac{\partial v(\mathbf{s}; \alpha)}{\partial \alpha_k} \left[ \mathcal{S}(-v(\mathbf{s}; \alpha) - F_c) - v(\mathbf{s}; \alpha) \frac{\partial \mathcal{S}(x)}{\partial x} \Big|_{x=-v(\mathbf{s}; \alpha) - F_c} \right] \quad (\text{S8})$$

which is simply the derivative of the linear expansion term multiplied by a factor in brackets due to the switching function. A similar relation can be obtained for the second derivatives in Eq. S6. We employ the averaged stochastic gradient descent algorithm [1] used previously in Refs. 2, 3. The iteration scheme involves both the average iterate,  $\bar{\alpha}^{(n)} = \frac{1}{n} \sum_{l=0}^n \alpha^{(l)}$  and the instantaneous iterate,  $\alpha^{(n)}$  which is updated according to

$$\alpha^{(n+1)} = \alpha^{(n)} - \mu \left[ \Omega'(\bar{\alpha}^{(n)}) + \Omega''(\bar{\alpha}^{(n)})[\alpha^{(n)} - \bar{\alpha}^{(n)}] \right], \quad (\text{S9})$$

where  $\mu$  is a fixed step size. In this work we consider only the diagonal terms of the Hessian matrix.

In practice the algorithm proceeds as follows: Initially the coefficients are set to zero, i.e.  $V(\mathbf{s}; \alpha^{(0)}) = 0$  and  $p^{(0)}(\mathbf{s})$  is a uniform distribution. We then iteratively update the coefficients  $\{\alpha_k\}$  every 1 ps according to Eq. S9 by sampling the gradient and Hessian from the biased simulation (sampling time of 1 ps). Every 50 bias potential iterations (or every 50 ps) we update the target distribution according to

$$p^{(j+1)}(\mathbf{s}) = \frac{\mathcal{S}(F^{(j+1)}(\mathbf{s}) - F_c)}{\int d\mathbf{s}' \mathcal{S}(F^{(j+1)}(\mathbf{s}') - F_c)} \quad (\text{S10})$$

where  $F^{(j+1)}(\mathbf{s}) = -v(\mathbf{s}; \alpha)$  is the current estimate of the FES within the region defined by  $F_c$  obtained using the previous target distribution  $p^{(j)}(\mathbf{s})$ . The updating of the target distribution is very similar to the one presented in Ref. 3. The iteration process of the bias potential and the target distribution is continued until the parameters  $\{\alpha_k\}$  are sufficiently converged. We note that the constant in  $v(\mathbf{s}; \alpha)$  ( $\alpha_0$  in the current case) is also periodically adjusted during the iteration process (generally at the same time as target distribution is updated) to make sure that  $V(\mathbf{s}; \alpha)$  goes properly to zero at the cutoff.

All of the results in this work were performed using the Fermi-type switching function of the form,

$$\mathcal{S}(-v(\mathbf{s}) - F_c) = \frac{1}{1 + e^{\lambda[-v(\mathbf{s}) - F_c]}}. \quad (\text{S11})$$

The parameter,  $\lambda$  is in units of inverse energy and determines how quickly the switching function goes to zero. Throughout this work, we have set  $\lambda = 1$  in units of  $[\text{kJ/mol}]^{-1}$ . The choice of the switching function is somewhat arbitrary, and other forms of  $\mathcal{S}(-v(\mathbf{s}) - F_c)$  could be used.

## S2. ALANINE DIPEPTIDE IN VACUUM COMPUTATIONAL DETAILS

In Fig. S1 we show the converged free energy surface obtained using the variational approach without any cutoff. Simulations were performed using the Amber99-SB force field [4] with GROMACS4.6.5 [5] patched with a private

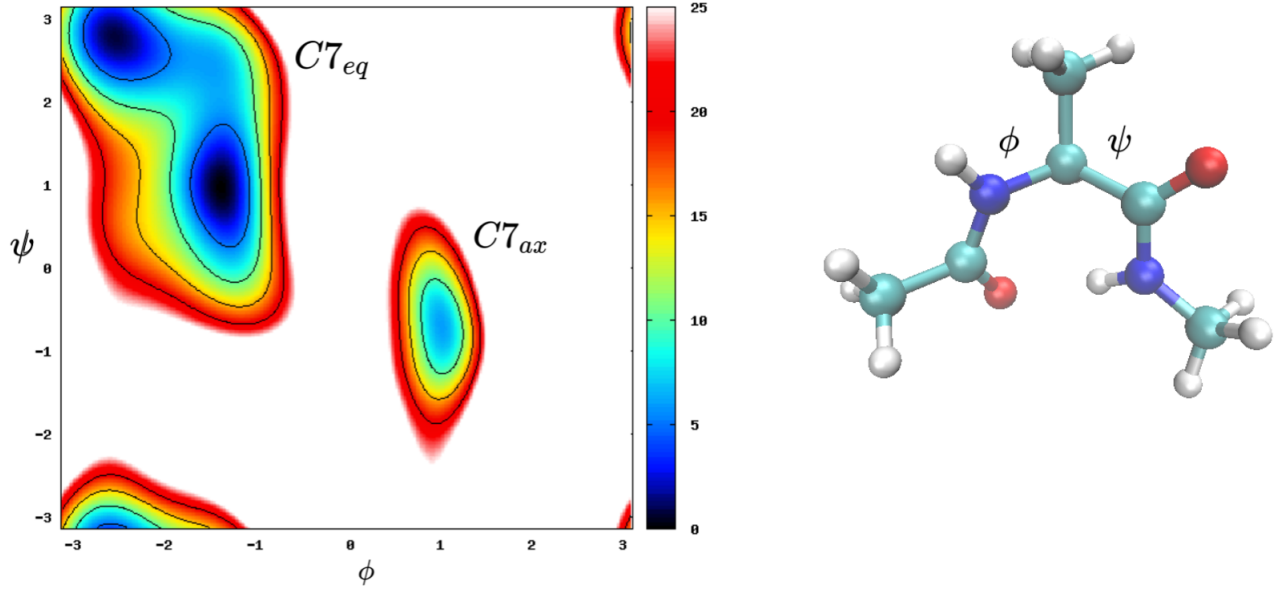

FIG. S1: Left: Reference free energy surface of alanine dipeptide in vacuum obtained using the variational method with no  $F_c$ . The minima are labeled according to the conventional name of the conformers,  $C7_{eq}$  and  $C7_{ax}$ . Right: The dihedral angles,  $(\phi, \psi)$  used as CV's for the alanine dipeptide molecule.

development implementation of the PLUMED2 plug-in [6]. We used a time step of 0.002 ps. Bonds were constrained using the LINCS algorithm [7], and the temperature was kept constant using the velocity rescaling thermostat [8]. For the well tempered metadynamics (WTMetaD) simulations, we used an initial Gaussian height of 1.25 kJ/mol, with a width of 0.25 rad for both CVs, and a deposition stride of 20 ps, which was used in reference [9]. We used a bias factor of 6 at 250 K.

### S3. VARIATIONAL PARAMETERS FOR ALANINE DIPEPTIDE IN VACUUM

For the optimization of the bias potential, we used a Fourier series,  $v(\mathbf{s}; \alpha) = \sum_k \alpha_k e^{i\mathbf{k} \cdot \mathbf{s}}$  with periodicity  $[-\pi, \pi]$ , and all coefficients initialized to zero. In practice, we consider real coefficients and use sine and cosine functions as the basis functions. The total number of basis functions is given by  $(2 \cdot M + 1)^d - 1$  where we use  $M = 6$  and thus have 168 variational coefficients in two dimensions. The coefficients were updated every 1 ps using Eq. S9 with a fixed step size of  $\mu = 0.05$ . The probability distribution,  $p(\mathbf{s})$  was updated every 50 ps. For the  $C7_{eq} \rightarrow C7_{ax}$  transition, we are only interested in first passage times, so the bias was constructed only in the well corresponding to the  $C7_{eq}$  state by optimizing the bias for only 1 ns, which is generally too short for a transition to the  $C7_{ax}$  state to occur during

the optimization. Fig. S2 shows the local estimate of  $F(\mathbf{s}) = -V(\mathbf{s})$  after 1 ns of optimization for various values of  $F_c$ . The resulting bias was used as a fixed bias for the first passage time calculation.

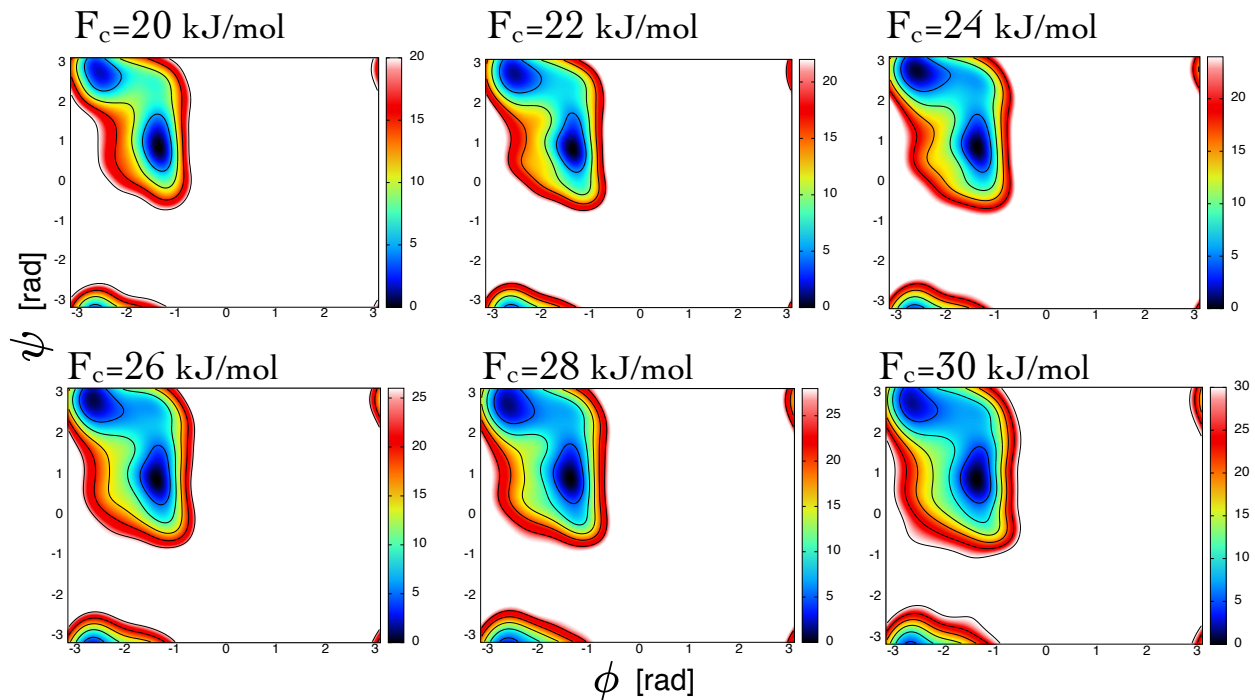

FIG. S2: Estimate of the free energy obtained from the negative of the bias,  $F(\mathbf{s}) = -V(\mathbf{s})$ , after 1 ns with variational parameters updated every 1 ps for increasing  $F_c$  values.

#### S4. EFFICIENCY COMPARED TO WELL TEMPERED METADYNAMICS

As stated in the main text, we performed a 1 ns optimization of the bias for a series of  $F_c$  values. During the optimization, the parameters were updated every 1 ps and  $p(\mathbf{s})$  was updated every 50 optimization steps. Subsequently, we used this bias in 60 independent trajectories and measured the first passage time (fpt) for the  $C_{7eq} \rightarrow C_{7ax}$  transition. The cumulative distribution function (CDF) is presented in the main text, and is compared to that obtained from WTMetaD. In Table S1 we show the total cumulative MD time required to obtain 60 crossing events for each  $F_c$  and for WTMetaD. This represents the computational time required to obtain the statistics presented in the main text. As can be seen in Table S1, the method is more efficient than WTMetaD for all  $F_c$  except for the lowest,  $F_c = 22$  kJ/mol. Even for the fastest case,  $F_c = 30$  kJ/mol, the 1 ns optimization is negligibly small compared

to the production time. Table S1 illustrates that if we have a good estimate of the barrier height, then the method gives an order of magnitude gain in efficiency over WTMetaD. However, even with a modest estimate of the barrier height, the method is more efficient or at least as efficient as WTMetaD.

TABLE S1: Comparison of Total MD Simulation Times for Obtaining 60 Barrier Crossing Events for Alanine Dipeptide in Vacuum at  $T = 300K$

| $F_c$ [kJ/mol] | optimization | production | total MD  |
|----------------|--------------|------------|-----------|
|                | time [ns]    | time [ns]  | time [ns] |
| 30             | 1.0          | 38.1       | 39.1      |
| 28             | 1.0          | 68.2       | 69.2      |
| 26             | 1.0          | 157.2      | 158.2     |
| 24             | 1.0          | 373.8      | 374.8     |
| 22             | 1.0          | 848.8      | 849.8     |
| WTMetaD        | NA           | 708.3      | 708.3     |

## S5. BENZOPHENONE IN WATER COMPUTATIONAL DETAILS

The structure of benzophenone in vacuum was optimized using the GAUSSIAN09 program package [10] with the B3LYP/6-31G\* basis set. Subsequently, the *ab-initio* Mulliken charges were computed using the HF/6-31G\* basis set. Partial charges were obtained from the GAUSSIAN output using antechamber with the RESP fitting procedure in AmberTools [11, 12]. We used the generalized AMBER (GAFF) [13, 14] force field parameters, and then manually stiffened the dihedral parameters for the  $\phi_1$  and  $\phi_2$  angles. In the final system, all dihedral angles are equivalent to the aromatic carbon dihedral parameters. The molecule was placed in a cubic box of length 3.46 nm with periodic boundary conditions and solvated with 993 TIP3P water molecules. Bonds to H atoms were constrained using the LINCS [15] and the SETTLE algorithms [16]. All simulations were carried out in the GROMACS4.6.5 simulation package [5] patched with our implementation of the variational method in PLUMED2 [6]. All simulations used a timestep of 0.002 ps. The temperature was kept constant with stochastic velocity rescaling [8], and the pressure was controlled using the Berendsen barostat. For long-range electrostatics, the particle-mesh Ewald method (PME) [17] was adopted.

# S6. VARIATIONAL PARAMETERS FOR BENZOPHENONE IN WATER

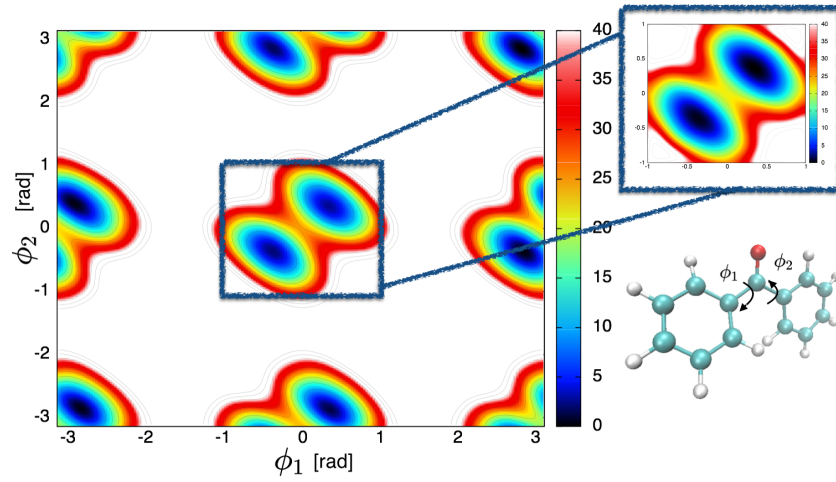

FIG. S3: Reference free energy surface of benzophenone and the highlighted region of interest obtained using Chebyshev polynomials over the range  $[-1 : 1]$ .

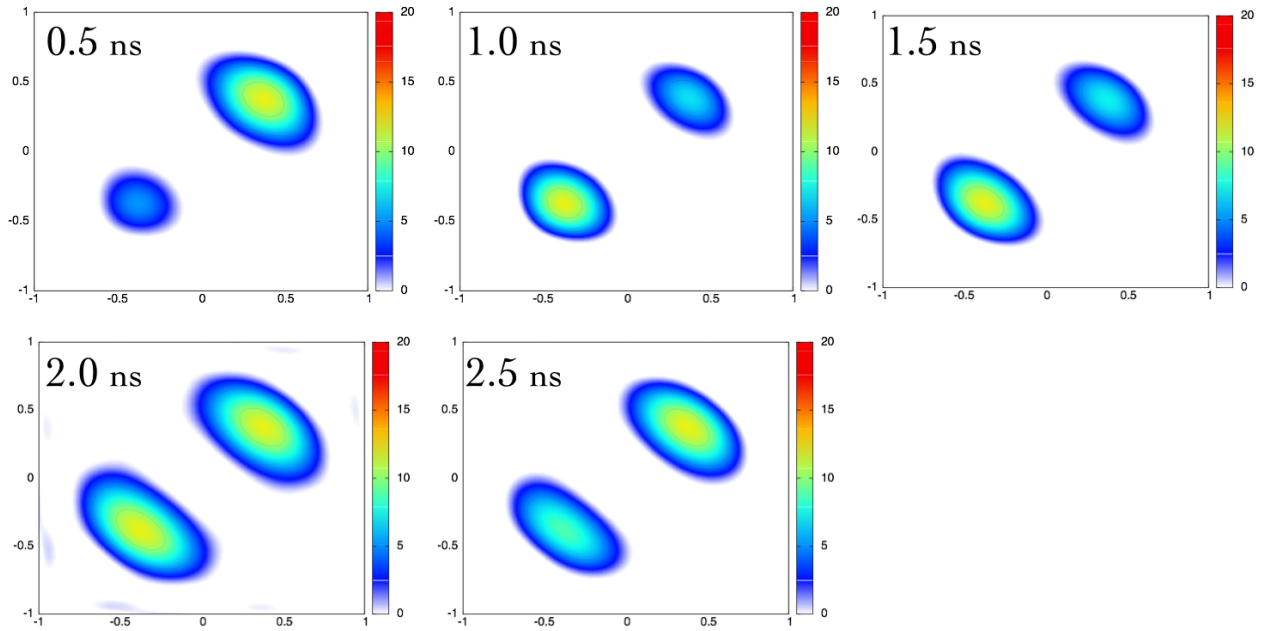

FIG. S4: Time series of the two dimensional bias for benzophenone during the optimization of the bias at  $T = 300K$  with  $F_c = 12$  kJ/mol.

TABLE S2: Comparison of Unrescaled and Rescaled Transition Times Obtained Using Static Biases from Figure S4

| optimization | unrescaled time        | unrescaled time        | rescaled time          | rescaled time          |
|--------------|------------------------|------------------------|------------------------|------------------------|
| MD time [ns] | A $\rightarrow$ B [ns] | B $\rightarrow$ A [ns] | A $\rightarrow$ B [ns] | B $\rightarrow$ A [ns] |
| 0.5          | $1.47 \pm 0.23$        | $0.24 \pm 0.06$        | $3.5 \pm 0.5$          | $3.0 \pm 0.7$          |
| 1.0          | $0.75 \pm 0.19$        | $1.05 \pm 0.20$        | $4.9 \pm 1.2$          | $3.7 \pm 0.7$          |
| 1.5          | $0.40 \pm 0.06$        | $0.87 \pm 0.13$        | $3.8 \pm 0.6$          | $3.6 \pm 0.5$          |
| 2.0          | $0.23 \pm 0.02$        | $0.18 \pm 0.02$        | $4.5 \pm 0.4$          | $3.7 \pm 0.3$          |
| 2.5          | $0.44 \pm 0.02$        | $0.23 \pm 0.01$        | $3.5 \pm 0.1$          | $3.5 \pm 0.1$          |

The free energy was obtained as a function of the  $\phi_1$  and  $\phi_2$  dihedral angles shown in the main text and below in Fig. S3. The CVs are periodic over the range  $[-\pi : \pi]$ , and the two dimensional FES over the entire range is shown in Fig. S3. The basic features of the FES repeat with a smaller periodicity; thus we investigate only the transitions between the two minima within the squared region of Fig. S3. We employ a basis set using a product of Chebyshev polynomials,

$$v(\mathbf{s}; \alpha) = \sum_{k_1=0}^{M_1} \sum_{k_2=0}^{M_2} \alpha_{k_1, k_2} \cdot T_{k_1}(s_1) \cdot T_{k_2}(s_2), \quad (\text{S12})$$

where  $T_k(\mathbf{s})$  are the Chebyshev polynomials of the first kind. The Chebyshev polynomials are defined in the range from  $[-1 : 1]$  to obtain the local FES around the two minima highlighted in Fig. S3. We used  $M_1 = M_2 = 8$  coefficients in the summation of Eq. S12 resulting in a total of  $(M+1)^d - 1 = 80$  variational coefficients. Coefficients were updated every 1 ps with a fixed stepsize of  $\mu = 0.01$ . To increase the sampling and ensure a stable optimization we used 4 multiple walkers with an  $F_c = 12$  kJ/mol to obtain the bias with the cutoff. The target distribution,  $p(s)$  was updated every 50 optimization steps. The total optimization of the bias was run for 2.5 ns; however, in Fig. S4 we show the bias obtained over the range 0.5 - 2.5 ns for the  $T = 300K$  case. As can be seen from Fig. S4, after this time, the bias is not fully converged and the height of the barrier is still different in the two basins. This is due to the fact that the walkers make a limited number of transitions between one well and another. Such events, although accelerated by the bias, are still relatively rare. It would thus require a very long time to fully converge the truncated bias; however, this is not necessary for the present purpose where the only requirement is that the bias fills the well only up to  $F_c$ , which it does by construction. The two apparent rates from  $A \rightarrow B$  and  $B \rightarrow A$  are different, but once



the rates are converted into physical time, they become equal as expected.

- 
- [1] F. Bach and E. Moulines, in *Advances in Neural Information Processing Systems 26*, edited by C. Burges, L. Bottou, M. Welling, Z. Ghahramani, and K. Weinberger (Curran Associates, Inc., Red Hook, NY, 2013), pp. 773–781.
  - [2] O. Valsson and M. Parrinello, *Phys. Rev. Lett.* **113**, 090601 (2014).
  - [3] O. Valsson and M. Parrinello, *J. Chem. Theory Comput.* **11**, 1996 (2015).
  - [4] V. Hornak, R. Abel, A. Okur, B. Strockbine, A. Roitberg, and C. Simmerling, *Proteins: Structure, Function, and Bioinformatics* **65**, 712 (2006).
  - [5] S. Pronk, S. Páll, R. Schulz, P. Larsson, P. Bjelkmar, R. Apostolov, M. R. Shirts, J. C. Smith, P. M. Kasson, D. van der Spoel, et al., *Bioinformatics* p. btt055 (2013).
  - [6] G. A. Tribello, M. Bonomi, D. Branduardi, C. Camilloni, and G. Bussi, *Comput. Phys. Commun.* **185**, 604 (2014).
  - [7] B. Hess, H. Bekker, H. J. Berendsen, J. G. Fraaije, et al., *J. Comput. Chem.* **18**, 1463 (1997).
  - [8] G. Bussi, D. Donadio, and M. Parrinello, *J. Chem. Phys.* **126**, 014101 (2007).
  - [9] P. Tiwary and M. Parrinello, *Phys. Rev. Lett.* **111**, 230602 (2013).
  - [10] M. Frisch, G. Trucks, H. B. Schlegel, G. Scuseria, M. Robb, J. Cheeseman, G. Scalmani, V. Barone, B. Mennucci, G. Petersson, et al., *Wallingford, CT* **19**, 227 (2009).
  - [11] C. I. Bayly, P. Cieplak, W. Cornell, and P. A. Kollman, *J. Phys. Chem.* **97**, 10269 (1993).
  - [12] J. Wang, W. Wang, P. A. Kollman, and D. A. Case, *J. Am. Chem. Soc.* **222**, U403 (2001).
  - [13] J. Wang, R. M. Wolf, J. W. Caldwell, P. A. Kollman, and D. A. Case, *J. Comput. Chem.* **25**, 1157 (2004).
  - [14] J. Wang, W. Wang, P. A. Kollman, and D. A. Case, *J. Mol. Graph. Model.* **25**, 247 (2006).
  - [15] B. Hess, *J. Chem. Theory Comput.* **4**, 116 (2008).
  - [16] S. Miyamoto and P. A. Kollman, *J. Comput. Chem.* **13**, 952 (1992).
  - [17] U. Essmann, L. Perera, M. L. Berkowitz, T. Darden, H. Lee, and L. G. Pedersen, *J. Chem. Phys.* **103**, 8577 (1995).
